# Supplementary material for: 3D Object Recognition By Corresponding and Quantizing Neural 3D Scene Representations
Source: arXiv:2010.16279 source file (2020-10-30)
Supplement: Supplementary file 1 [file 9_suppl_FAQ.tex]

\section{Frequently asked questions}
\label{sec: faq_supp}
\begin{itemize}
    \item \textbf{How are the prototypes initialized? How is K (number of prototypes) chosen?:} We want to ensure the prototypes are diverse at initialization time. An exemplar only gets assigned as a prototype if its feature distance to the already-initialized prototypes is higher than a threshold. In Figure 3(main paper), we show how varying K affects the prototype learning: for the method to work well, K needs to be large enough to cover the object variability in the dataset. In all other experiments, we set K=50.
    
    \item \textbf{How well does prototype matching work with occluded/incomplete objects?:} Our view prediction loss in Section 3.1(main paper) ensures that given an input RGB-D view, the network completes the input information by learning to imagine the occluded and missing object information. The 3D feature maps, inferred from a single view, encode complete object information, thus it is possible to match them with complete prototypes.
    
    \item \textbf{Are the resized maps of objects of different sizes similar?:} Yes, they are similar. The feature maps are resized using trilinear interpolation both during object to prototype matching and during correspondence mining.
    
    \item \textbf{Why use axis-aligned boxes? Does this affect the rotation-aware feature matching?:} Our goal is to use our model for 3D perception in the wild. Since 3D object boxes are not available in the real world, we need to use a publicly available 2D object detector to get initial boxes using triangulation. Since the 2D object detector produces axis-aligned 2D boxes, we end up generating 3D boxes which are axis-aligned. Our rotation-aware feature matching in Section 3.2(main paper) is designed to work with axis-aligned boxes, so it is not affected. In Figure \ref{fig:supp_rotational_align}, we show our method can retrieve the correct orientation.

    \item \textbf{Are the detections not matching to prototypes penalized?:} No, we do not consider these detections as negatives. As mentioned in main paper, we select our negative proposals using a 3D center-surround saliency check. The hope is that these false positive proposals will eventually become true positives, once the 3D detector improves via iterative learning.
    
    \item \textbf{How is the detector initialized? Why not use 3D connected components/semantic segmentation?:} The 3D detector is initialized by training on pseudo-ground-truth 3D bounding boxes obtained from a pre-trained 2D object detector, FasterRCNN, by triangulating 2D box detections from multiple views. Since the 2D detector works well in finding objects in the real scene, it provides a good start for our detectors for self-improvement.

    Getting object 3D boxes using connected components requires removing the planar surface (with RANSAC) from below the object, so that the connected component only covers the object of interest. Empirically, we found this step to be fragile, and the method fails in cluttered scenes. Semantic segmentation also requires triangulating 2D segmentations to get 3D GT. In practice, we found publicly available segmentation models to be less reliable than 2D object proposal models.
    
    \item \textbf{Why not use GT 3D detections in simulation?:} Our goal is to use our system for real world self-supervised 3D perception, thus we do not want to rely on simulated 3D groundtruth.

    \item \textbf{Why is feature compressibility important?:} Our goal is to organize (i.e., compress) the visual world in a set of frequently occurring prototypes which allows object recognition to happen in a few-shot setting. Our model compresses well, as it does not waste representation in modelling different 3D rotations and scales of objects

\end{itemize}
